# Supplementary material for: Interpolation between Convolution and Attention via K-Nearest Neighbors
Source: arXiv:2606.14725 source file (2026-05-31)
Supplement: Supplementary file 1 [file AppendixA.tex]

% Appendix A
